# Supplementary material for: Modelling Populations of Interaction Networks via Distance Metrics
Source: arXiv:2206.09995 source file (2022-06-20)
Supplement: Supplementary file 1 [file x-appendix.tex]

\appendix

\input{supplement/sample_spaces}
\input{supplement/simulations}

\begin{figure}
    \centering
    \includegraphics[page=2, width=0.85\linewidth]{img/data analysis/foursquare_analysis_main.pdf}
    \caption{Paths of our point estimate $\hat{\E}^m$ for the Foursquare data, alongside those of $\E^{(1)}$ and $\E^{(2)}$, its two nearest neighbours. The remaining paths can be seen in \Cref{fig:fsq_sim_est1,fig:fsq_sim_est3}.}
    \label{fig:fsq_sim_est2}
\end{figure}

\begin{figure}
    \centering
    \includegraphics[page=3, width=0.85\linewidth]{img/data analysis/foursquare_analysis_main.pdf} 
    \caption{Paths of our point estimate $\hat{\E}^m$ for the Foursquare data, alongside those of $\E^{(1)}$ and $\E^{(2)}$, its two nearest neighbours. The remaining paths can be seen in \Cref{fig:fsq_sim_est1,fig:fsq_sim_est2}.}
    \label{fig:fsq_sim_est3}
\end{figure}
