# Supplementary material for: Modelling Populations of Interaction Networks via Distance Metrics
Source: arXiv:2206.09995 source file (2022-06-20)
Supplement: Supplementary file 2 [file 0-main.tex]

% \appendixpageoff
% \appendixtitleoff
\newpage

\begin{appendices}
    % \appendix 
    \setcounter{page}{1}  % Reset page numbers
    \setcounter{section}{0}
        % Labels for sections

    \crefalias{section}{supp}
    \crefalias{subsection}{supp}
    \crefalias{subsubsection}{supp}
    
    \section*{Supplementary Material}
    
    \vspace{0.5cm}
    
    \input{supplement/entropy_montonicity}

    \input{supplement/iexchange_algorithm}
    
    \input{supplement/mcmc_details}
    
    \input{supplement/inference_sim}

    \input{supplement/data_analysis}
    
%    \putbib\\

    \newpage
    \input{supplement/pseudocode}
    
\end{appendices}
