# Supplementary material for: Modelling Populations of Interaction Networks via Distance Metrics
Source: arXiv:2206.09995 source file (2022-06-20)
Supplement: Supplementary file 3 [file imcmc_background.tex]

% \begin{algorithm}[h]
% 	\SetAlgoLined
% 	\KwIn{target density $p(\theta | \mathbf{x})$}
% 	\KwIn{density $p(u|\theta)$ and a sampler from $p(u|\theta)$}
% 	\KwIn{involution $f(\theta,u)$, i.e. $f^{-1}(\theta,u) = f(\theta,u)$}	
% 	initialise $\theta$\;
% 	\For{$i=1,\dots,n$}{
% 		sample $u \sim p(u|\theta)$ \\
% 		propose $(\theta^\prime, u^\prime) = f(x, u)$ \\
% 		sample $\mathbf{y}$ (approximately) from $p(\mathbf{y}|\theta^\prime)$ via iMCMC \\
% 		$\alpha = \min\left\{1, \frac{p(\theta^\prime) \gamma(\mathbf{x} | \theta^\prime) \gamma(\mathbf{y}| \theta) p(u^\prime| \theta^\prime) }{p(\theta) \gamma(\mathbf{x} | \theta) \gamma(\mathbf{y}| \theta^\prime)  p(u| \theta)}\left| \frac{\partial f(\theta, u)}{\partial (\theta, u)}\right|\right\}$ \\
% 		$\theta_i = \begin{cases}
% 			\theta^\prime & \text{with probability } \alpha \\
% 			\theta & \text{with probability } (1-\alpha)
% 		\end{cases}$ \\
% 		$\theta \leftarrow \theta_i$
		
% 	}
% 	\caption{Double iMCMC }
% 	\label{alg_sup:double_imcmc}
% \end{algorithm}
